# Supplementary material for: A Structure-Agnostic Multi-Objective Evolutionary Weight-Sharing Compression Framework for Deep Neural Networks
Source: arXiv:2501.03095 source file (2026-11-24)
Supplement: Supplementary file 1 [file appendix.tex]

\documentclass[lettersize,journal]{IEEEtran}
\usepackage{times}
\usepackage{graphicx}
\usepackage{amssymb}
\usepackage{url,hyperref}
\usepackage{booktabs}
\usepackage{multirow}
\usepackage{subcaption}
\usepackage{algorithm,algpseudocode}
\usepackage{amsmath}
\usepackage{adjustbox}
\usepackage{mathtools}
\usepackage{lipsum} 
\usepackage{textcomp}
\usepackage{stfloats}
\usepackage{verbatim}
\usepackage{graphicx}
\usepackage{cite}
\begin{document}
\onecolumn
\newpage
\appendix[Pseudo code]
\input{pseudocode_linspace}
% \newpage
\appendix[Cumulative Results]
\input{cifars_tables}
\input{imagenet_tables}
\end{document}
